# Supplementary material for: Autonomous Option Invention for Continual Hierarchical Reinforcement Learning and Planning
Source: arXiv:2412.16395 source file (2024-12-20)
Supplement: Supplementary file 1 [file appendix.tex]

This paper presents a novel approach for autonomous option invention and transfer, a challenging open problem for hierarchical and continual RL.

\section{Selection of Domains and Task Details}

We chose test domains that are well established as challenging for state-of-the-art RL 
\citep{
andreas2017modular,
kokel2021reprel, jin2022creativity} with considerably larger maps than those used in most prior investigations. In each domain, we generated a continual stream of 20 randomly sampled tasks, varying in initial states, goal states, and reward functions. We evaluated each approach on its ability to solve the entire continual RL problem within a given budget for each task. The chosen tasks are particularly difficult due to their long horizons and sparse rewards.

% Moreover, unlike latent state abstractions, e.g., where an abstract state may be characterized by the similarity across output of the inner layers of a neural network, the abstraction computed in this approach is easy to interpret, in other words it has a well-defined definition and meaning. 

 We detail the specific differences among the tasks in each randomly generated continual RL problem for the selected domains. These tasks share the same state and action spaces but vary in their objectives as follows. 

\begin{itemize}
    \item In \textbf{Maze World} \citep{ramesh2019successor}, the agent must navigate from a randomly selected starting location to a randomly chosen goal within a large 24$\times$24 continuous map, avoiding randomly placed wall obstacles. It can move in four cardinal directions, with a 0.8 probability of successful movement and a 0.1 probability of slipping to an adjacent cell. The agent receives a reward of 500 upon reaching the goal and -1 elsewhere.

 \item In \textbf{Four Rooms} \citep{sutton1999between}, the agent navigates within and between rooms, moving through hallways to reach a randomly chosen goal from a random starting location within a 33$\times$33 continuous map. The effects of actions due to stochasticity and the reward structure are the same as in Maze World.

\item In \textbf{Office World} \cite{icarte2018using}, the agent starts at a random location, tasked with collecting coffee and mail from specific locations and delivering them to a randomly chosen desk within an 11$\times$15 office. The agent receives a reward of 500 upon successfully completing a task and 0 elsewhere.

\item In \textbf{Taxi World} \cite{dietterich2000hierarchical},  
the taxi starts at a random location, must pick up a passenger from a randomly selected pickup location and drop them off at a randomly chosen destination. The map of size 30$\times$30 features four specific pickup and dropoff locations. The agent is penalized with a -100 reward for illegal pick or dropoff actions, and it receives a reward of 500 for successfully completing the task of delivering the passenger to its destination, with a -1 penalty for other moves.

\item 
In \textbf{Minecraft} \cite{andreas2017modular},  
the agent starts at a random location in a 22$\times$22 map, needs to gather wood from randomly selected forest locations to craft a stick, and then mine resources like iron or stone to build either a stone or an iron axe. The tasks are randomly chosen to build either a stone or iron axe, so the agent must identify and collect the necessary resources. Movement incurs a cost of -1, and the agent receives a reward of 500 for crafting the correct axe.

 \end{itemize}
For training option policies in our approach, we provide the agent an intrinsic sparse reward of 500 upon reaching abstract terminations of options.

\section{Selection of Baselines}
 We evaluated existing work to select the best performing baselines on the selected problems, focusing on those that do not rely on hand-engineered abstractions or action hierarchies. Extensive evaluation by \cite{dadvar2023conditional}
% (henceforth ``DNS23'') 
showed that \catrl{} dominated Qlearning \cite{watkins1992q} and state-of-the-art deep RL approaches like DQN \cite{mnih2013playing}, PPO \cite{schulman2017proximal}, and A2C \cite{mnih2016asynchronous}. As a result, we selected \catrl{} as a suitable baseline for comparison. We compared with Option-Critic \cite{bacon2017option} as it is a state-of-the-art approach for end-to-end learning of transferable options. Lastly, we also compared with PPO \cite{schulman2017proximal}, a state-of-the-art DRL approach for learning latent representations to solve RL problems.

% The presented approach \alg{} does not need to predefine the number of options as Option-Critic does. \alg{} uses parameters 
% $n_{check}$, $t_{succ}$, and cap $k$ similar to \catrlalg{}.
% $n_{check}$ is the interval of number of episodes at which abstraction is evaluated for refinement, $t_{succ}$ is the threshold of success rate, and the cap $k$ is the maximum number of unstable states that can be refined in each refinement. $t$ denotes the abstraction distance threshold between pruned-CATs and $t'$ denotes the abstract state distance within the CAT used to invent novel CAT-options. $\epsilon$ is the abstract state proximity threshold used during planning over option library to find a plan for a new problem.
% $f$ is the factor used to control the abstraction distance heuristic of edges retained and is set to $\frac{1}{4}$ for all domains. 
% $n_{eval}$ is the number of episodes for which the learned greedy policy is evaluated, which is set to 100 for all our experiments. 

\begin{table*}[h!]
% [htbp!]
    \centering
    \begin{tabular}{@{}|l|c|c|c|c|@{}}
\toprule

        Hyperparameters & \alg{} & Option-Critic & \catrlalg{} & PPO  \\
        \midrule
                Task budget in timesteps $(\gH)$ & 1.5M & 1.5M & 1.5M & 1.5M \\
        % Threshold ($t_{succ}$) & 0.9 & 0.9 & 0.9 \\
        %  Abstraction update episode interval ($n\_check$) & 100 & 100 & 100 \\     
        % Evaluation episodes ($n\_eval$) & 100 & 100& 100 \\
        % Learning rate $\alpha$ & & & & & & &  \\
        % Exploration rate & 1.0 & $-$ & 1.0  \\
        Exploration decay & 0.997  & 0.997 & 0.997 & $-$ \\
            % Exploration decay for options & 0.994 & $-$ & $-$ & $-$\\
        Minimum exploration rate & 0.05 & 0.05  & 0.05  & $-$ \\
        % Exploration fraction & $-$  & $-$ & 0.1 \\
        % Learning rate $(\alpha)$ & 0.05  & 1e-4 & 1e-4 \\ 
        Learning rate $(\alpha)$ & 0.05 & 0.05 & 0.05 & 3e-4\\
        Discount factor $(\gamma)$ & 0.99  & 0.99 & 0.99 & 0.99\\
        Episode stepmax & 500 & 500 & 500 & 500 \\
        % Option episode Stepmax & 250 & $-$ & $-$ \\
        % Option training steps threshold & 250K & $-$ & $-$ \\
        Cap on abstraction refinement $(k_\emph{cap})$ & 2 & $-$ & 5 & $-$\\
         Context-specific distance  threshold $(\delta_{\emph{thre}})$ & 0 & $-$ & $-$ & $-$\\
        Context-independent distance  threshold $(\sigma_{\emph{thre}})$ & 0.95 & $-$ & $-$ & $-$\\
        % Cap on abstraction refinement for options $k_\emph{cap}$ & 2 & $-$ & $-$\\
        Factor to adjust stepmax for options $(s_\emph{factor})$ & 10 & $-$ & $-$ & $-$\\
        Maximum episodes to halt option training $(e_\emph{max })$ & 500 & $-$ & $-$ & $-$\\
        Number of options & $-$ & 8  &$-$ & $-$ \\
        Temperature & $-$ & 0.001  & $-$  & $-$  \\
         Termination regularization & $-$ & 0.01  & $-$  & $-$  \\ Entropy regularization & $-$ & 0.01  & $-$  & $-$  \\
        Generalized Advantage Estimator  (gae\_lambda)& $-$ & $-$  &$-$ & 0.95 \\
        Steps to run per update (n\_steps) & $-$ & $-$  &$-$ & 2048 \\
         % Batch size & $-$ & $-$  &$-$ & 64 \\
         Entropy coefficient (ent\_coef) & $-$ & $-$  &$-$ & 0.0 \\
         Value function coefficient (vf\_coef) & $-$ & $-$  &$-$ & 0.5 \\ 
         Maximum gradient clipping (max\_grad\_norm) & $-$ & $-$  &$-$ & 0.5\\ 
        \bottomrule
    \end{tabular}
    \caption{Hyperparameters used in Maze World.}
    \label{tab:tab1}
\end{table*}

\begin{table*}[h!]
    \centering
    \begin{tabular}{@{}|l|c|c|c|c|@{}}
\toprule
        Hyperparameters & \alg{} & Option-Critic & \catrlalg{} & PPO  \\
        \midrule
        Task budget in timesteps $(\gH)$ & 2M & 2M & 2M & 2M \\
        Exploration decay & 0.998  & 0.998 & 0.998 & $-$ \\
        % Exploration decay for options & 0.998 & $-$ & $-$ & $-$\\
        Minimum exploration rate & 0.05 & 0.05  & 0.05  & $-$ \\
        Learning rate $(\alpha)$ & 0.05 & 0.05 & 0.05 & 3e-4\\
        Discount factor $(\gamma)$ & 0.999  & 0.999 & 0.999 & 0.999\\
        Episode stepmax & 800 & 800 & 800 & 800 \\
        Cap on abstraction refinement $(k_\emph{cap})$ & 2 & $-$ & 5 & $-$\\
         Context-specific distance  threshold $(\delta_{\emph{thre}})$ & 0 & $-$ & $-$ & $-$\\
        Context-independent distance  threshold $(\sigma_{\emph{thre}})$ & 0.95 & $-$ & $-$ & $-$\\
        Factor to adjust stepmax for options $(s_\emph{factor})$ & 10 & $-$ & $-$ & $-$\\
        Maximum episodes to halt option training $(e_\emph{max })$ & 500 & $-$ & $-$ & $-$\\
        Number of options & $-$ & 8  &$-$ & $-$ \\
        Temperature & $-$ & 0.001  & $-$  & $-$  \\
         Termination regularization & $-$ & 0.01  & $-$  & $-$  \\ Entropy regularization & $-$ & 0.01  & $-$  & $-$  \\
        Generalized Advantage Estimator  (gae\_lambda)& $-$ & $-$  &$-$ & 0.95 \\
        Steps to run per update (n\_steps) & $-$ & $-$  &$-$ & 2048 \\
         % Batch size & $-$ & $-$  &$-$ & 64 \\
         Entropy coefficient (ent\_coef) & $-$ & $-$  &$-$ & 0.0 \\
         Value function coefficient (vf\_coef) & $-$ & $-$  &$-$ & 0.5 \\ 
         Maximum gradient clipping (max\_grad\_norm) & $-$ & $-$  &$-$ & 0.5\\ 
        \bottomrule
    \end{tabular}
    \caption{Hyperparameters used in Four Rooms World.}
    \label{tab:tab2}
\end{table*}

\begin{table*}[h!]
% [htbp!]
    \centering
    \begin{tabular}{@{}|l|c|c|c|c|@{}}
\toprule
        Hyperparameters & \alg{} & Option-Critic & \catrlalg{} & PPO  \\
        \midrule
        Task budget in timesteps $(\gH)$ & 4M & 4M & 4M & 4M \\
        Exploration decay & 0.999  & 0.999 & 0.999 & $-$ \\
        % Exploration decay for options & 0.998 & $-$ & $-$ & $-$\\
        Minimum exploration rate & 0.05 & 0.05  & 0.05  & $-$ \\
        Learning rate $(\alpha)$ & 0.05 & 0.05 & 0.05 & 3e-4\\
        Discount factor $(\gamma)$ & 1  & 1 & 1 & 1\\
        Episode stepmax & 1000 & 1000 & 1000 & 1000 \\
        Cap on abstraction refinement $(k_\emph{cap})$ & 2 & $-$ & 5 & $-$\\
         Context-specific distance  threshold $(\delta_{\emph{thre}})$ & 0 & $-$ & $-$ & $-$\\
        Context-independent distance  threshold $(\sigma_{\emph{thre}})$ & 1 & $-$ & $-$ & $-$\\
        Factor to adjust stepmax for options $(s_\emph{factor})$ & 4 & $-$ & $-$ & $-$\\
        Maximum episodes to halt option training $(e_\emph{max })$ & 200 & $-$ & $-$ & $-$\\
        Number of options & $-$ & 8  &$-$ & $-$ \\
                Temperature & $-$ & 0.001  & $-$  & $-$  \\
         Termination regularization & $-$ & 0.01  & $-$  & $-$  \\ Entropy regularization & $-$ & 0.01  & $-$  & $-$  \\
        Generalized Advantage Estimator  (gae\_lambda)& $-$ & $-$  &$-$ & 0.95 \\
        Steps to run per update (n\_steps) & $-$ & $-$  &$-$ & 2048 \\
         % Batch size & $-$ & $-$  &$-$ & 64 \\
         Entropy coefficient (ent\_coef) & $-$ & $-$  &$-$ & 0.0 \\
         Value function coefficient (vf\_coef) & $-$ & $-$  &$-$ & 0.5 \\ 
         Maximum gradient clipping (max\_grad\_norm) & $-$ & $-$  &$-$ & 0.5\\ 
        \bottomrule
    \end{tabular}
    \caption{Hyperparameters used in Taxi World.}
    \label{tab:tab3}
\end{table*}

\begin{table*}[h!]
% [htbp!]
    \centering
    \begin{tabular}{@{}|l|c|c|c|c|@{}}
\toprule
        Hyperparameters & \alg{} & Option-Critic & \catrlalg{} & PPO  \\
        \midrule
        Task budget in timesteps $(\gH)$ & 4M & 4M & 4M & 4M \\
        Exploration decay & 0.9991  & 0.9991 & 0.9991 & $-$ \\
        % Exploration decay for options & 0.999 & $-$ & $-$ & $-$\\
        Minimum exploration rate & 0.05 & 0.05  & 0.05  & $-$ \\
        Learning rate $(\alpha)$ & 0.05 & 0.05 & 0.05 & 1e-2\\
        Discount factor $(\gamma)$ & 0.99  & 0.99 & 0.99 & 0.99\\
        Episode stepmax & 800 & 800 & 800 & 800 \\
        Cap on abstraction refinement $(k_\emph{cap})$ & 5 & $-$ & 5 & $-$\\
         Context-specific distance  threshold $(\delta_{\emph{thre}})$ & 0 & $-$ & $-$ & $-$\\
        Context-independent distance  threshold $(\sigma_{\emph{thre}})$ & 1 & $-$ & $-$ & $-$\\
        Factor to adjust stepmax for options $(s_\emph{factor})$ & 10 & $-$ & $-$ & $-$\\
        Maximum episodes to halt option training $(e_\emph{max })$ & 200 & $-$ & $-$ & $-$\\
        Number of options & $-$ & 8  &$-$ & $-$ \\
                Temperature & $-$ & 0.001  & $-$  & $-$  \\
         Termination regularization & $-$ & 0.01  & $-$  & $-$  \\ Entropy regularization & $-$ & 0.01  & $-$  & $-$  \\
        Generalized Advantage Estimator  (gae\_lambda)& $-$ & $-$  &$-$ & 0.95 \\
        Steps to run per update (n\_steps) & $-$ & $-$  &$-$ & 2048 \\
         % Batch size & $-$ & $-$  &$-$ & 64 \\
         Entropy coefficient (ent\_coef) & $-$ & $-$  &$-$ & 0.0 \\
         Value function coefficient (vf\_coef) & $-$ & $-$  &$-$ & 0.5 \\ 
         Maximum gradient clipping (max\_grad\_norm) & $-$ & $-$  &$-$ & 0.5\\ 
        \bottomrule
    \end{tabular}
    \caption{Hyperparameters used in Office World.}
    \label{tab:tab4}
\end{table*}

\begin{table*}[h!]
% [htbp!]
    \centering
    \begin{tabular}{@{}|l|c|c|c|c|@{}}
\toprule
        Hyperparameters & \alg{} & Option-Critic & \catrlalg{} & PPO  \\
        \midrule
        Task budget in timesteps $(\gH)$ & 3M & 3M & 3M & 3M \\
        Exploration decay & 0.999  & 0.999 & 0.999 & $-$ \\
        % Exploration decay for options & 0.999 & $-$ & $-$ & $-$\\
        Minimum exploration rate & 0.05 & 0.05  & 0.05  & $-$ \\
        Learning rate $(\alpha)$ & 0.05 & 0.05 & 0.05 & 3e-4 \\
        Discount factor $(\gamma)$ & 1  & 1 & 1 & 1\\
        Episode stepmax & 1000 & 1000 & 1000 & 1000 \\
        Cap on abstraction refinement $(k_\emph{cap})$ & 2 & $-$ & 5 & $-$\\
         Context-specific distance  threshold $(\delta_{\emph{thre}})$ & 0 & $-$ & $-$ & $-$\\
        Context-independent distance  threshold $(\sigma_{\emph{thre}})$ & 1 & $-$ & $-$ & $-$\\
        Factor to adjust stepmax for options $(s_\emph{factor})$ & 10 & $-$ & $-$ & $-$\\
        Maximum episodes to halt option training $(e_\emph{max })$ & 200 & $-$ & $-$ & $-$\\
        Number of options & $-$ & 8  &$-$ & $-$ \\
                Temperature & $-$ & 0.001  & $-$  & $-$  \\
         Termination regularization & $-$ & 0.01  & $-$  & $-$  \\ Entropy regularization & $-$ & 0.01  & $-$  & $-$  \\
        % Network architecture & $-$ & $-$  &$-$ & 64$\times$64 \\
        Generalized Advantage Estimator  (gae\_lambda)& $-$ & $-$  &$-$ & 0.95 \\
        Steps to run per update (n\_steps) & $-$ & $-$  &$-$ & 2048 \\
         % Batch size & $-$ & $-$  &$-$ & 64 \\
         Entropy coefficient (ent\_coef) & $-$ & $-$  &$-$ & 0.0 \\
         Value function coefficient (vf\_coef) & $-$ & $-$  &$-$ & 0.5 \\ 
         Maximum gradient clipping (max\_grad\_norm) & $-$ & $-$  &$-$ & 0.5\\ 
        \bottomrule
    \end{tabular}
    \caption{Hyperparameters used in Minecraft.}
    \label{tab:tab5}
\end{table*}

\section{Hyperparameter Details}
We implemented our approach \alg{} in Python. The code is provided with instructions to run along with this appendix, and will make it public post publication. 
For baselines, we used the open-source code available for Option-Critic \footnote[1]{https://github.com/lweitkamp/option-critic-pytorch}, \catrlalg{} \footnote[2]{https://github.com/AAIR-lab/CAT-RL.git}, and used standard architectures for PPO from Stable-Baselines3 \footnote[3]{https://github.com/DLR-RM/stable-baselines3} by \cite{raffin2019stable}. 

A key advantage of our approach, \alg{}, over most baseline methods is that it requires only five additional hyperparameters beyond standard RL parameters (e.g., decay, learning rate) and is robust to most parameter values, as long as they are intuitively set. In contrast, SOTA deep RL methods need extensive tuning, significant effort in network architecture design, and are highly sensitive to hyperparameter values. Unlike Option-Critic, \alg{} does not require the number of options to be specified in advance. For Option-Critic, we parametrize the intra-option policies  with Boltzmann distributions and the terminations with sigmoid functions. Tables ~\ref{tab:tab1} (Maze World), ~\ref{tab:tab2} (Four Rooms), ~\ref{tab:tab3} (Taxi World),  ~\ref{tab:tab4} (Office World), and ~\ref{tab:tab3} (Minecraft) show the used hyperparameters for \alg{} and all baselines on these domains.

The parameters used by \alg{} are: $\delta_{\emph{thre}}$ and $\sigma_{\emph{thre}}$ are distance thresholds used for option invention, $k_\emph{cap}$ is the cap on the number of abstract states refined in option-specific CATs, $s_\emph{factor}$ is a scaling factor for adaptively adjusting the stepmax for training option policies (stepmax for an option is set to $s_\emph{factor}$ * length of recent successful trajectory), and $e_\emph{max}$ is the maximum episode limit for learning an option’s policy before halting training to do replanning.  Our approach uses $k_\emph{cap}$ parameter for controlling abstraction refinement for options, as used by \catrl{} for the entire problem. Throughout our experiments, we intuitively set $\delta_{\emph{thre}} = 0$ and $\sigma_{\emph{thre}} \sim 1$. These values are robust across domains, preventing options from being too small or numerous. We use a limited set of values for other parameters to minimize hyperparameter tuning. All parameters are set to the same values across a continual stream of tasks for a domain.
